# Supplementary material for: Luminosity and Beam-Induced Background Studies for the Cool Copper Collider
Source: arXiv:2403.07093 source file (2024-05-24)
Supplement: Supplementary file 1 [file Luminosity_BIB_C3_Supplemental.pdf]

# Supplemental Material
## Luminosity and Beam-Induced Background Studies for the Cool Copper Collider


Dimitrios Ntounis,* Emilio Alessandro Nanni,† and Caterina Vernieri‡
*SLAC National Accelerator Laboratory, 2575 Sand Hill Road, Menlo Park, California 94025, USA*
*Stanford University, 450 Jane Stanford Way, Stanford, California 94305, USA*


(Submitted: Friday 24 May 2024)


## I. LUMINOSITY SPECTRA FOR C$^3$-550 BEAM PARAMETER OPTIMIZATION

We evaluate the effect of modifications in the bunch length $\sigma_z^*$ by comparing the luminosity spectrum for C$^3$-550 with the PS1 beam parameters to the ones for various bunch length and waist shift values, assuming a vertical emittance of 14 nm. The results are presented in Figure 1a and indicate a broadening of the luminosity spectrum for $\sigma_z^* = 70$ µm. This broadening implies a more significant BIB, which would deteriorate detector performance. For this reason, the bunch length is retained at its PS1 value of 100 µm, as explained in the main text.

We additionally investigated the effect of modifications in the horizontal emittance $\epsilon_x^*$ by comparing the luminosity spectra for $\epsilon_x^*$ =900, 1100 nm with respect to the baseline beam configuration PS1, as shown in Figure 1b. We notice that for $\epsilon_x^* = 900$ nm, the tails of the luminosity spectrum are enhanced, whereas for $\epsilon_x^* = 1100$ nm, the tails are comparable to the PS1 case, while still achieving luminosity gain close to $\sqrt{s_0} = 550$ GeV. This motivated the choice of an intermediate value of $\epsilon_x^* = 1000$ nm for the PS2 C$^3$ beam configuration, as explained in the main text.

## II. LUMINOSITY SCANS FOR BEAM OFFSET

In Section IV E of the main text, the normalized luminosity $\mathscr{L}/\mathscr{L}$ as a function of the relative vertical beam offset $\Delta y/\sigma_y^*$ was shown in Fig. 8b for various colliders. In Figure 2a, we additionally show the absolute luminosity values, allowing one to compare the luminosity values for various colliders at a given beam offset. Finally, in Figures 2b,2c, the same information is plotted for the relative horizontal offset $\Delta x/\sigma_x^*$.

## III. ADDITIONAL DISTRIBUTIONS OF BACKGROUND PARTICLES

The distributions of the energy and longitudinal boost of the produced $e^+e^-$ background pairs were shown for various collider configuration in Figure 11 of Section V of the main text. The distributions for the longitudinal $p_z$ and transverse $p_T$ momenta of these particles are given for completeness in Figures 3a and 3b respectively.


* dntounis@slac.stanford.edu
† nanni@slac.stanford.edu
‡ caterina@slac.stanford.edu

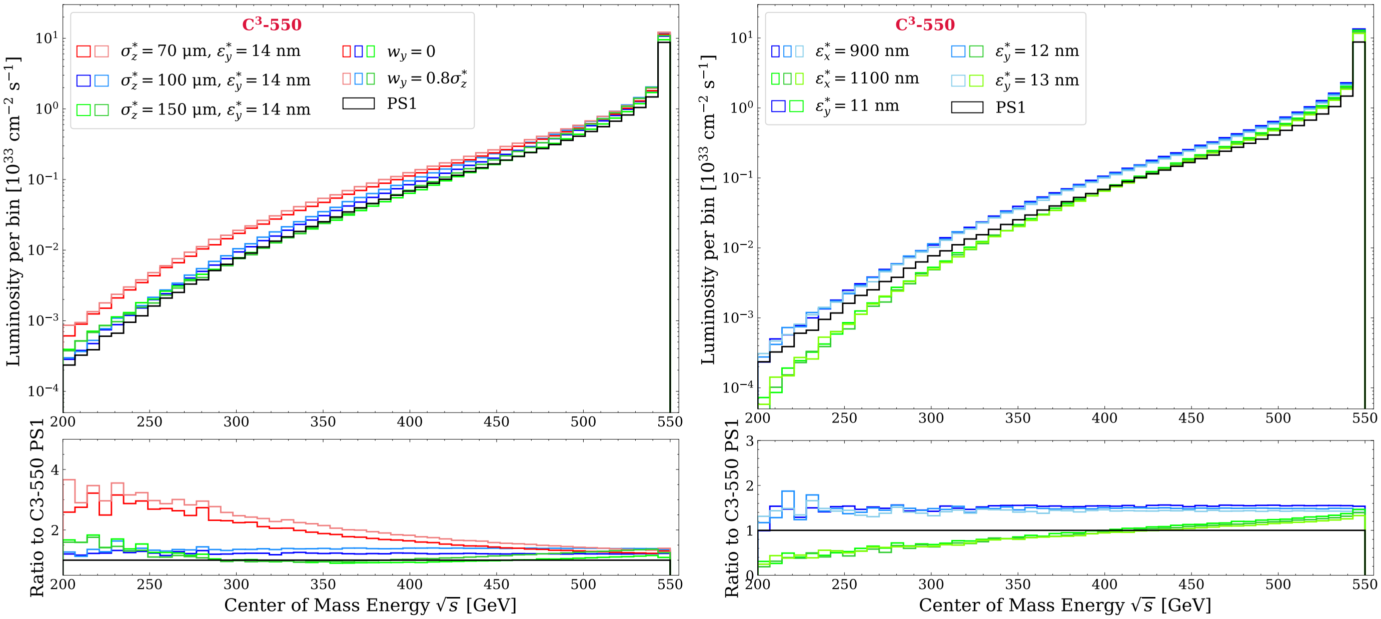


(a) (b)

FIG. 1: Luminosity spectra for C$^3$-550 (a) for bunch lengths $\sigma_z^*$ of 70, 100 and 150 µm, vertical waist shifts $w_y$ of 0 and $0.8\sigma_z^*$ and a vertical emittance $\epsilon_y^* = 14$ nm and (b) for horizontal emittances $\epsilon_x^* = 900$ and 1100 nm and vertical emittances $\epsilon_y^* = 11, 12$ and 13 nm. In (b), bunch lengths $\sigma_z^* = 100$ µm and waist shifts $w_y = 80$ µm have been assumed in all six cases. The luminosity spectrum for the PS1 parameter set is also given for comparison. All other beam parameters are kept to their nominal values.

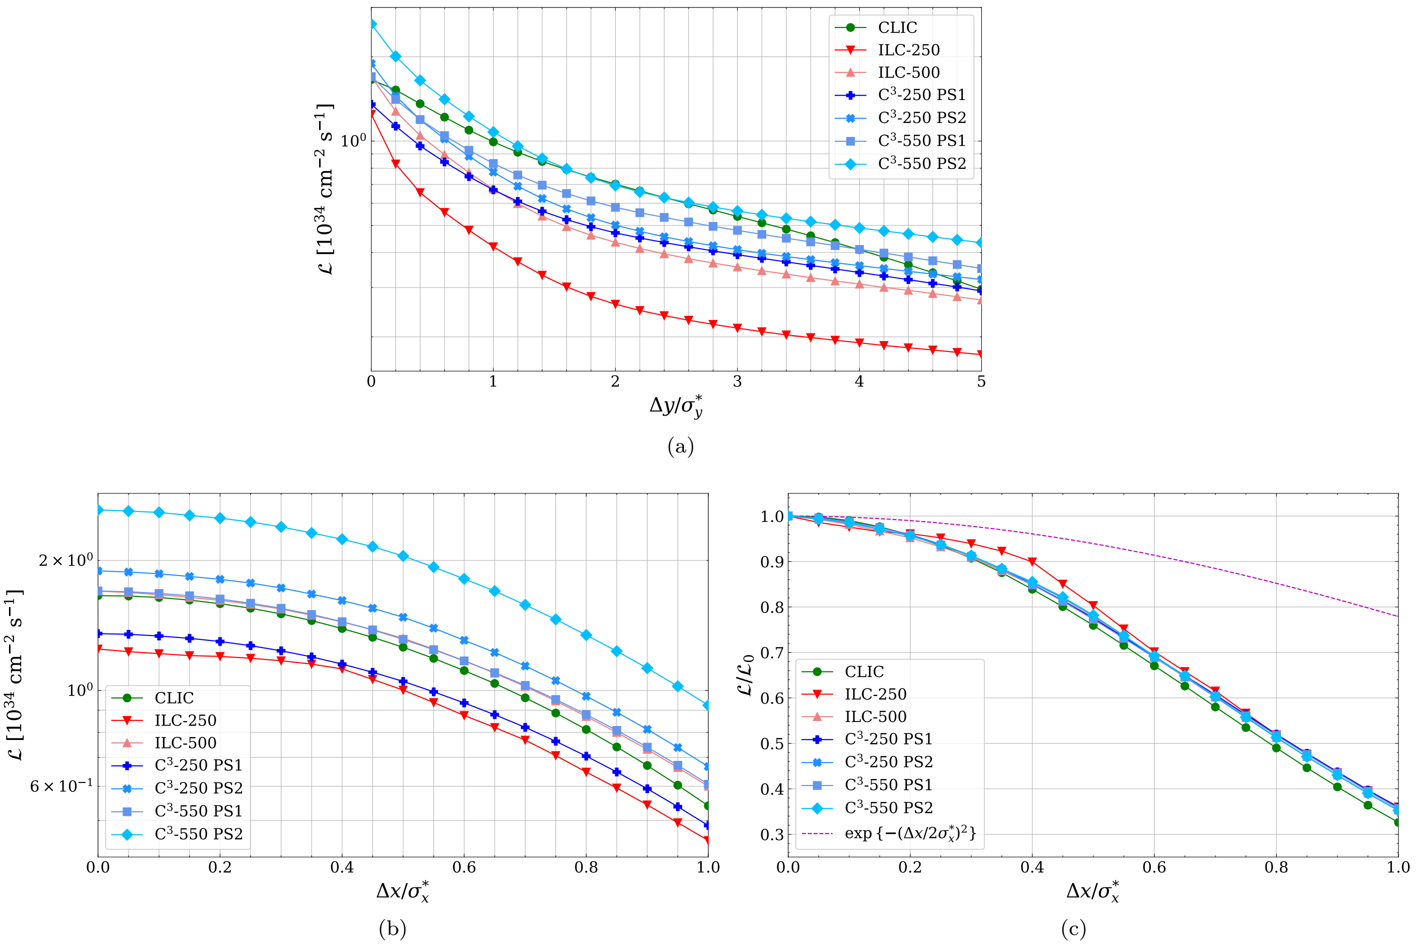


FIG. 2: Luminosity scans for CLIC, ILC and $C^3$ as a function of the horizontal beam offset $\Delta x$. In (a), the absolute luminosity numbers are given, whereas in (b) the luminosity for each collider is normalized with respect to its value when assuming zero offset.

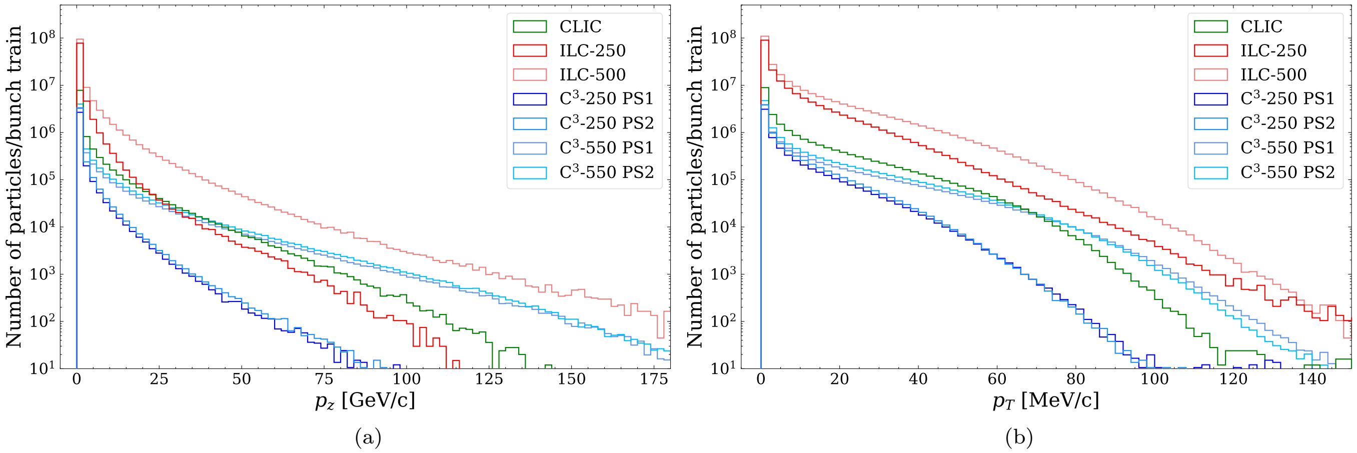


FIG. 3: Distributions of (a) the longitudinal momentum and (b) the transverse momentum of the incoherent $e^+e^-$ pairs for various linear collider proposals. Each distribution has been normalized to the expected number of incoherent pair particles per bunch train $N_{\rm incoh} \cdot n_b$.
